# Supplementary material for: Registering Neural 4D Gaussians for Endoscopic Surgery
Source: arXiv:2407.20213 source file (2024-07-29)
Supplement: Supplementary file 1 [file 6_appendix.tex]

\section*{APPENDIX}

Appendixes should appear before the acknowledgment.
